# Supplementary material for: Extract Free Dense Labels from CLIP
Source: arXiv:2112.01071 source file (2022-07-27)
Supplement: Supplementary file 4 [file tab-supp-zero-shot-new.tex]

\begin{table}[t]
\footnotesize
\centering
{
\def\sp{SPNet}
\def\spc{SPNet-C}
\def\zs{ZS3Net}
\def\cag{CaGNet}

\def\zsst{ZS3Net}
\def\cagst{CaGNet}

\def\denseclipplus{\methodname+}
\def\voc{\textbf{PASCAL-VOC}}
\def\context{\textbf{PASCAL-Context}}
\def\stuff{\textbf{COCO-Stuff}}
\newcommand{\better}[1]{\textcolor{ForestGreen}{(+#1)}}
\newcommand{\worse}[1]{\textcolor{BrickRed}{(-#1)}}

\caption{\inlinesection{Zero-shot segmentation performances (pAcc \& mAcc)}}
\label{tab:supp-zero-shot}
\setlength{\tabcolsep}{1pt}

\begin{tabular}{l ccc c ccc c ccc}
    \noalign{\medskip}
    \toprule
    \multirow{2}{*}{Method} & \multicolumn{3}{c}{\voc}     && \multicolumn{3}{c}{\stuff}       && \multicolumn{3}{c}{\context} \\
                            &  pAcc\textsubscript{(S)} & pAcc\textsubscript{(U)} & pAcc 
                            && pAcc\textsubscript{(S)} & pAcc\textsubscript{(U)} & pAcc 
                            && pAcc\textsubscript{(S)} & pAcc\textsubscript{(U)} & pAcc \\
    % \midrule
    % Inductive \\
    \midrule
    \sp                     & \textbf{94.8} & 0.0  & 76.9    && 65.6 & 1.7 & 51.3        && \ph & \ph & \ph \\
    \spc                    & 88.8 & 29.6 & 77.6    && 61.8 & 24.5 & 53.4       && \ph & \ph & \ph \\
    \zs                     & 93.0 & 21.5 & 79.4    && 64.3 & 22.8 & 54.7       && 53.5 & 58.6 & 52.8 \\
    \cag                    & 89.5 & 43.0 & 80.7    && 65.6 & 25.5 & 56.6       && 55.2 & 66.8 & 56.6 \\
    % \midrule
    % Transductive \\
    \midrule
    % \spst                   & \ph & \ph & \ph       && \ph & \ph & \ph          && \ph & \ph & \ph \\
    \zsst                   & 91.9 & 34.1 & 81.0    && 65.8 & 24.9 & 56.3       && 46.8 & 70.2 & 49.5 \\
    \cagst                  & 87.0 & 58.6 & 81.6    && \textbf{65.9} & 26.7 & 56.8       && \ph & \ph & \ph \\
    % \strict                 & \ph & \ph & \ph       && \ph & \ph & \ph          && \ph & \ph & \ph \\
    \denseclipplus          & 94.6 & \textbf{91.4} & \textbf{94.0}
                            && 64.2 & \textbf{79.4} & \textbf{67.6}
                            && \textbf{73.9} & \textbf{82.3} & \textbf{74.8} \\
                            & \worse{0.2}  & \better{32.8} & \better{12.4}    
                            && \worse{1.7}  & \better{52.7} & \better{10.8}        
                            && \better{18.7} & \better{12.1} & \better{18.2} \\
    \midrule
    Fully Sup.        & \ph & \ph & 94.0        && \ph & \ph & 68.1            && \ph & \ph & 74.8 \\
    \bottomrule
\end{tabular}

\vspace{10pt}

\begin{tabular}{l ccc c ccc c ccc}
    \toprule
    \multirow{2}{*}{Method} & \multicolumn{3}{c}{\voc}     && \multicolumn{3}{c}{\stuff}       && \multicolumn{3}{c}{\context} \\
                            &  mAcc\textsubscript{(S)} & mAcc\textsubscript{(U)} & mAcc 
                            && mAcc\textsubscript{(S)} & mAcc\textsubscript{(U)} & mAcc 
                            && mAcc\textsubscript{(S)} & mAcc\textsubscript{(U)} & mAcc \\
    % \midrule
    % Inductive \\
    \midrule
    \sp                     & \textbf{94.6} & 0.0  & 70.9    && 50.3 & 0.0  & 45.9         && \ph & \ph & \ph \\
    \spc                    & 87.9 & 23.9 & 71.9    && 46.3 & 16.1 & 43.6         && \ph & \ph & \ph \\
    \zs                     & 87.7 & 15.8 & 73.5    && 50.4 & 27.0 & 48.4         && 23.8 & 43.2 & 27.0 \\
    \cag                    & 88.7 & 39.4 & 76.4    && 50.7 & 27.0 & 48.5         && 35.7 & 49.8 & 36.8 \\
    % \midrule
    % Transductive \\
    \midrule
    % \spst                   & \ph & \ph & \ph       && \ph & \ph & \ph           && \ph & \ph & \ph \\
    \zsst                   & 85.7 & 26.4 & 73.8    && 50.4 & 27.2 & 48.6        && 32.3 & 57.1 & 36.4 \\
    \cagst                  & 83.9 & 50.7 & 75.6    && 50.6 & 27.3 & 48.5        && \ph & \ph & \ph \\
    % \strict                 & \ph & \ph & \ph       && \ph & \ph & \ph           && \ph & \ph & \ph \\
    \denseclipplus          & 93.7 & \textbf{92.6} & \textbf{93.4}
                            && \textbf{50.8} & \textbf{72.4} & \textbf{52.7}
                            && \textbf{55.4} & \textbf{80.0} & \textbf{59.5} \\
                            & \worse{0.9}  & \better{41.9} & \better{17.0}    
                            && \better{0.1}  & \better{45.1} & \better{4.1}        
                            && \better{19.7} & \better{22.9} & \better{22.7} \\
    \midrule
    Fully Sup.        & \ph & \ph & 93.4        && \ph & \ph & 53.0            && \ph & \ph & 59.5 \\
    \bottomrule
\end{tabular}

}
\end{table}
